# Supplementary material for: TexVocab: Texture Vocabulary-conditioned Human Avatars
Source: arXiv:2404.00524 source file (2024-03-31)
Supplement: Supplementary file 1 [file X_suppl.tex]

\clearpage
\maketitlesupplementary
\setcounter{page}{1}

\section{OverView}
In Sec.~\ref{sec:S1}, we display more results of the synthesized avatar and geometric avatar. In Sec.~\ref{sec:S2} and Sec.~\ref{sec:S3}, we present more implementation details and how we conduct experiments, respectively. 

\section{More Results}
\label{sec:S1}
\subsection{Animation Results}
\hspace{0.422cm}Fig.~\ref{fig:figX1} shows more animation results of different datasets. Fig.~\ref{fig:figX2} displays animation results of different method on AIST++~\cite{li2021ai} dataset. The comparisons against results from PoseVocab and results from NeRF MLP with pose further demonstrate the generalization of our method. Fig.~\ref{fig:figX3} displays more anination results of different encoding methods(global-pose embedding, joint-structured embedding, body-part-wise embedding) on AMASS Dataset~\cite{mahmood2019amass}. For more animation results and comparisons against other methods such as ARAH~\cite{wang2022arah}, TAVA~\cite{li2022tava} and PoseVocab~\cite{li2023posevocab}, please refer to the supplementary videos.

\subsection{Geometric Results}
\hspace{0.422cm}Benefiting from VolSDF~\cite{yariv2021volume}, our method can also produce detailed geometric results as shown in Fig~\ref{fig:fig9}. The geometry results can also serve as priors to sample points near the surface in rendering to accelerate the training procedure.

\section{Implementation Details}
\label{sec:S2}

\subsection{Network Architecture}
\hspace{0.422cm}In our method, we use a CNN as the image encoder to extract features of the texture images, and we use a NeRF MLP to decode the 3D character. The architecture of the NeRF MLP is shown in Fig.~\ref{fig:fig10}. For the image encoder, following PixelNeRF~\cite{yu2021pixelnerf}, we use the ResNet34~\cite{he2016deep} backbone pre-trained on ImageNet for our experiments. Features are extracted prior to the first 3 pooling layers, upsampled using bilinear interpolation, and concatenated to form latent vectors of size 256 aligned to each pixel. Actually, changing the backbone of the network does not make much difference to the rendering results.

The number of nearest key body parts in KNN is $K = 4$, the number of key body parts equals to $0.3 \times T_1$, which can cover most of the appearances of training poses. And the resolution of the obtained texture images is 512 $\times$ 512. For the amount of training frames $T_1$, please refer to Sec.~\ref{sec:S31}.

\begin{figure}[t]
  \centering
  %\fbox{\rule{0pt}{1.5in} \rule{0.9\linewidth}{0pt}}
  %\includegraphics[scale=0.1]{fig/pipeline_07(1).jpg}
  \includegraphics[width=1.0\linewidth]{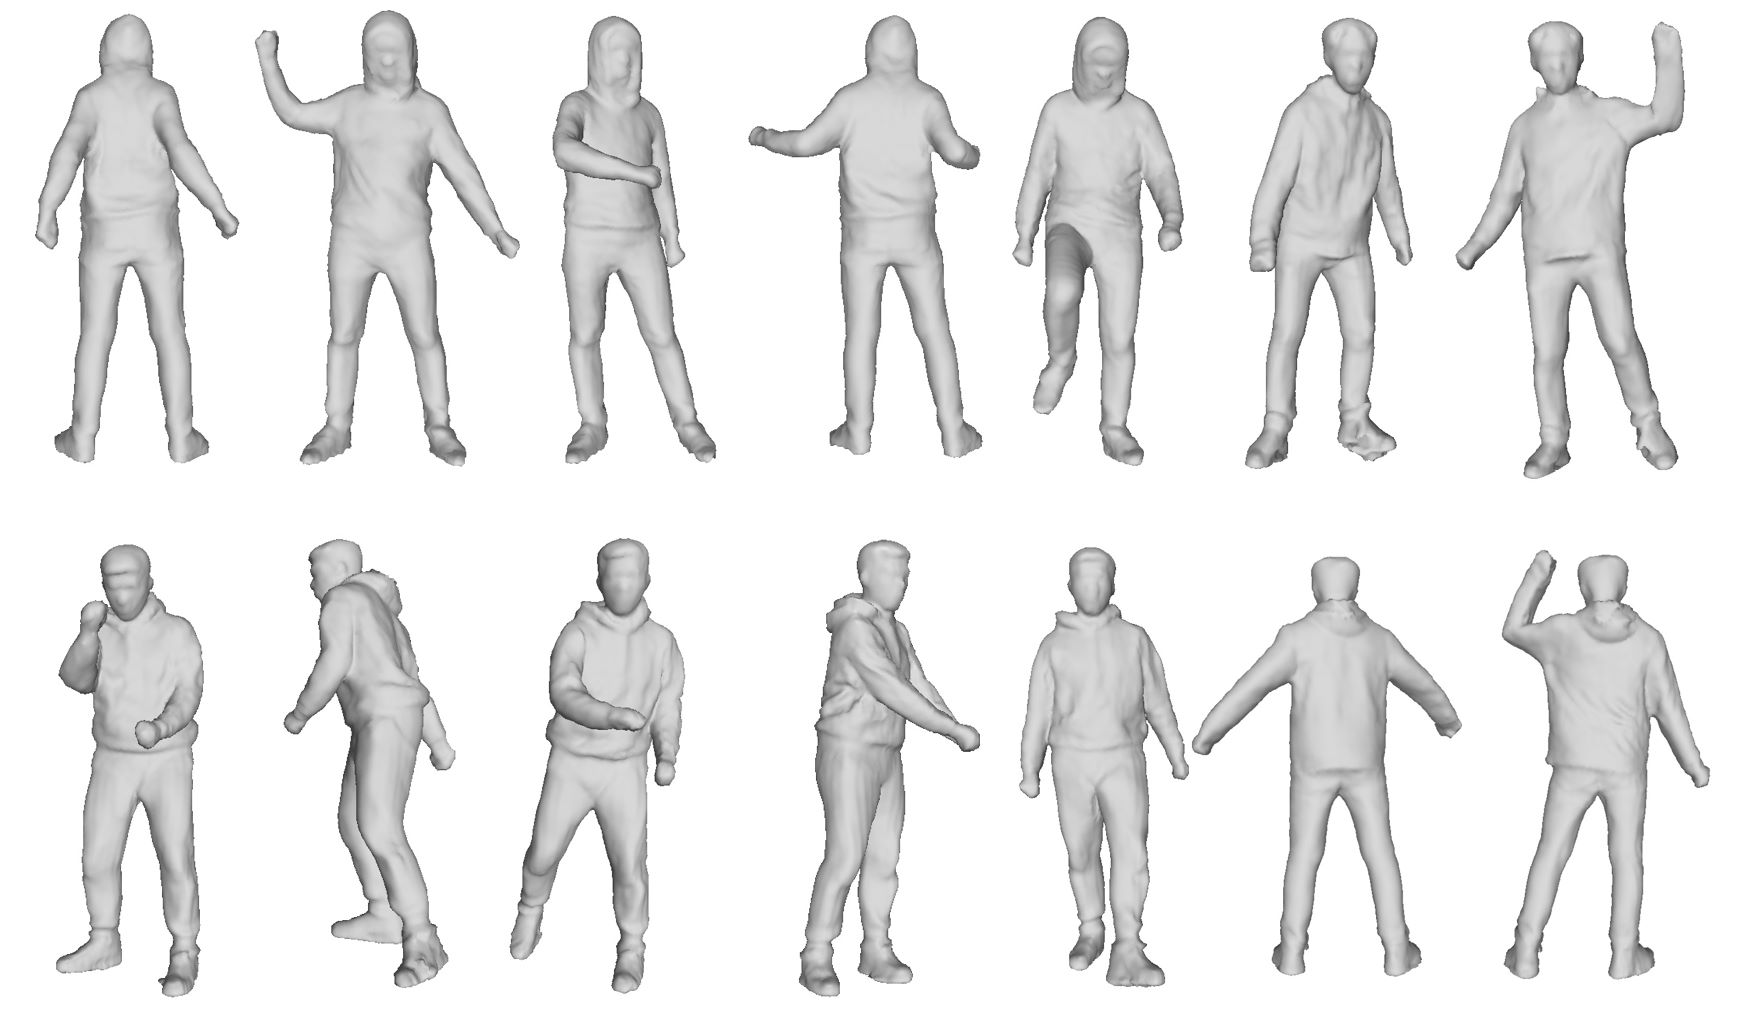}
   \caption{Geometric results of our method.}
   \label{fig:fig9}
\end{figure}

\begin{figure*}[htb]
  \centering
  %\fbox{\rule{0pt}{1.5in} \rule{0.9\linewidth}{0pt}}
  %\includegraphics[scale=0.1]{fig/pipeline_07(1).jpg}
  \includegraphics[width=1.0\linewidth]{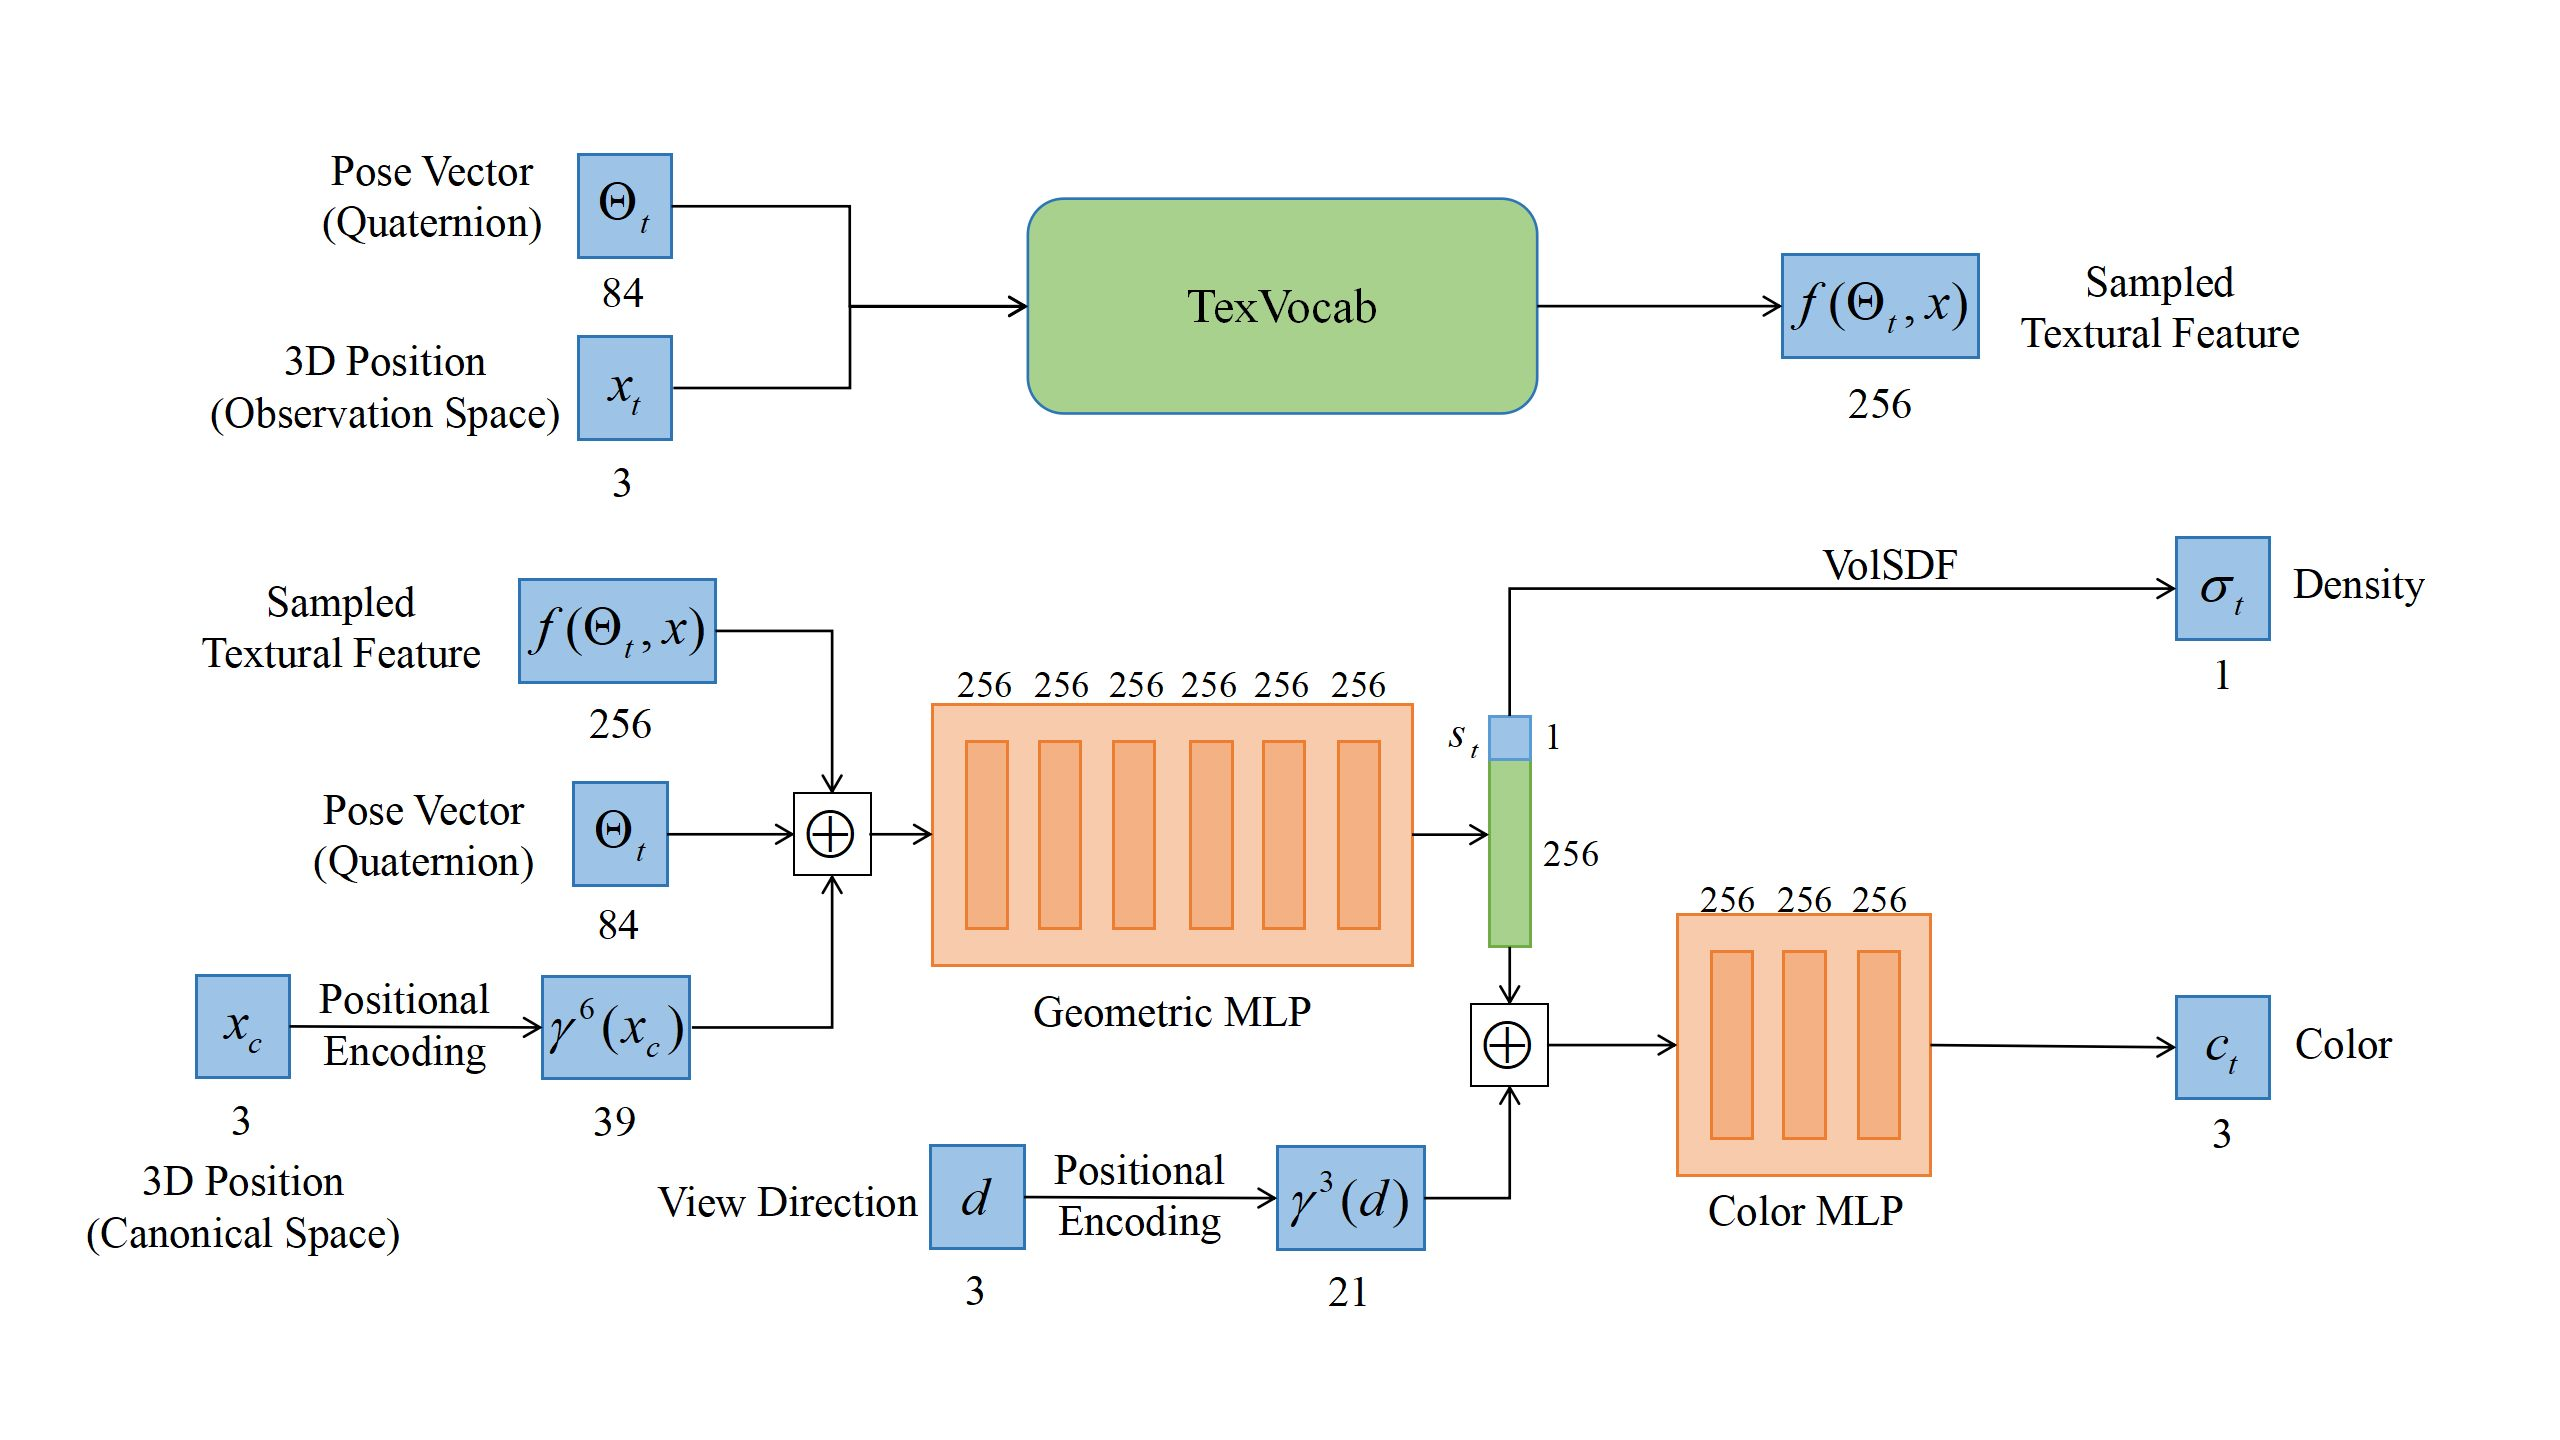}
   \caption{Architecture of our network.}
   \label{fig:fig10}
\end{figure*}

\subsection{Comparisons}
\hspace{0.422cm}For animation results of ARAH~\cite{wang2022arah}, TAVA~\cite{li2022tava}, AniNeRF~\cite{peng2021animatable} and PoseVocab~\cite{li2023posevocab}, we use the code released by authors. For results of NeuralActor~\cite{liu2021neural}, we borrow the results reported in the technical paper and presented in the video.

\section{Experimental Details}
\label{sec:S3}
\subsection{Datasets}
\label{sec:S31}
\hspace{0.422cm}In our experiments, we use 6 sequences of multi-view videos from THUman4.0 dataset~\cite{zheng2022structured}, ZJU-MoCap dataset~\cite{peng2021neural} and DeepCap dataset~\cite{habermann2020deepcap} for training and evaluation. We also use AMASS dataset~\cite{mahmood2019amass} and AIST++ dataset~\cite{li2021ai} for novel pose syhthesis. 

{\bf THUman4.0 Dataset.} We use sequence 'subject00', 'subject01' and 'subject02' in THUman4.0 Dataset~\cite{zheng2022structured}, which are all captured from 24 cameras, and contain 2500, 5060 and 3110 frames respectively. Each frame also provides SMPL-X~\cite{pavlakos2019expressive} registration. We use the first 2000 frames of all the cameras for training, and the rest are for testing.

{\bf ZJU-MoCap Dataset.} We use sequence 'CoreView\_313', 'CoreView\_394' in ZJU-MoCap Dataset~\cite{peng2021neural}. 
\label{exp_detail}. 'CoreView\_313' is captured by 21 cameras, while 'CoreView\_394' is captured by 23 cameras. Each frame provides SMPL~\cite{2015SMPL} registration. We both use the former 500 frames of all the cameras for training.

{\bf DeepCap Dataset.} We use sequence 'lan' in DeepCap Dataset~\cite{habermann2020deepcap}, which is captured from 11 cameras and contains around 33600 training frames and around 14200 testing frames. Each frame provides SMPL-X~\cite{pavlakos2019expressive} registration. We use all the cameras and sample every 10 frames in the training set for training, {i.e.}, the training dataset contains about 3360 poses. 
%Notice that although the dataset provides ground-truth texture maps, we do not use it for constructing texture vocabulary. Instead, we use back-projection to gather all the image evidence and obtain texture images since ground-truth texture images usually require a large number of cameras or even human resources, while other datasets in our experiments do not provide such conditions.

{\bf Testing Dataset.} We use several sequences from AMASS~\cite{mahmood2019amass} and AIST++~\cite{li2021ai} dataset for novel pose syhthesis to evaluate the generalization of our method.

\subsection{Training Loss}
\hspace{0.422cm} The training losses include a color loss, a
perceptual loss, a mask loss and the Eikonal loss.

{\bf Color Loss.} Color loss measures the MSE loss between the rendered image and ground-truth pixel colors:
\begin{equation}
	\begin{split}		 
 \mathcal{L}_{color}=\sum\nolimits_{r \in \mathcal{R}} \Vert \mathcal{C}(r) - \mathcal{C^*}(r) \Vert_2^2
	\end{split}
 \label{eq:loss1}
\end{equation}
where$\mathcal{R}$ is the set of sampled rays from the rendered view, and $\mathcal{C}(r)$ and $\mathcal{C^*}(r)$ are the rendered and true pixel colors, respectively.

{\bf Mask Loss.} Mask loss measures the MAE loss between the mask of rendered image and ground-truth:
\begin{equation}
	\begin{split}		 
 \mathcal{L}_{mask}=\sum\nolimits_{r \in \mathcal{R}} \Vert \mathcal{M}(r) - \mathcal{M^*}(r) \Vert_2^2
	\end{split}
 \label{eq:loss2}
\end{equation}
where $\mathcal{M}(r)$ and $\mathcal{M^*}(r)$ are the rendered and ground-truth mask values, respectively. The mask loss supervises the occupancy values of the rendered pixel.

{\bf Eikonal Loss.} Eikonal loss~\cite{gropp2020implicit} encourages the geometry fields to approximate a true signed distance function~\cite{yariv2021volume}:
\begin{equation}
	\begin{split}		 
\mathcal{L}_{eikonal} = \mathbb{E}(\Vert \nabla_x s(x,f(\Theta,x)) \Vert_2^2 - 1 )
	\end{split}
 \label{eq:loss3}
\end{equation}
where $s(\cdot)$ is the MLP-based function that maps a 3D position $x_c$ and pose feature $f(\Theta,x_c)$ to the SDF value.

{\bf Perceptual Loss.} The perceptual loss $\mathcal{L}_{perceptual}$ is widely used in NeRF training~\cite{li2023posevocab, zheng2022structured,zheng2023avatarrex}, which leads to better recovery of high-frequency details like the clothed wrinkles and thin lines~\cite{zhang2018unreasonable}. We choose VGGNet as the backbone to calculate the learned perceptual image patch similarity (LPIPS):
\begin{equation}
	\begin{split}		 
 \mathcal{L}_{color}=\sum\nolimits_{p \in \mathcal{P}} \Vert VGG(\mathcal{C}(r)) - VGG(\mathcal{C^*}(r)) \Vert_2^2
	\end{split}
 \label{eq:loss4}
\end{equation}
where $\mathcal{P}$ is the set of sampled patches from the rendered view, and $\mathcal{C}(r)$ and $\mathcal{C^*}(r)$ are the rendered and true patch colors, respectively.

Finally, we calculate the weight sum to optimize the network:
\begin{equation}
	\begin{split}		\mathcal{L}&=\lambda_{color}\mathcal{L}_{color}+\lambda_{mask}\mathcal{L}_{mask}\\&+\lambda_{perceptual}\mathcal{L}_{perceptual}+\lambda_{eikonal}\mathcal{L}_{eikonal}
	\end{split}
 \label{eq:loss_total}
\end{equation}
where the $\lambda s$ are loss weights.

\subsection{Training Details}
\hspace{0.422cm}We train the network using the Adam~\cite{kingma2014adam} optimizer with a batch size of 4 for 40 epochs. The initial learning rate is $5 \times 10^{-4}$ and decays by multiplying 0.9 every 20k iterations. The training procedure takes about 1 $\sim$ 2.5 days on 4 RTX 3090 cards varying different multi-view video sequences. 
The training procedure contains three stages.
In the first stage, we set $\lambda_{color} = 1$, $\lambda_{mask} = 1$, $\lambda_{eikonal} = 0.1$ and $\lambda_{perceptual} = 0$ during the first 6 epochs. We randomly sample 1024 rays on the training views, 80$\%$ of which are inside the mask image. For each ray, we sample 64 points within the SMPL bounding box. Under the supervision of the mask and color losses, a plausible geometry for each training frame can be learned.
Then we extract 3D meshes using Marching Cubes~\cite{we1987marching} for all the training frames by querying the SDF value of each voxel in a coarse 3D volume that contains the posed human, and then render depth maps of all the training frames. 
In the following training procedure, we use depth-guided sampling by only sampling 32 points near the surface based on the rendered depth map. The depth-guided sampling strategy not only accelerates the training process, but also encourages the network to focus on modeling the dynamic appearance of valid regions.
In the second stage, from the 6th to the 20th epoch, we set Eikonal loss to 0 for faster training.
In the third stage, we sample patches with a resolution of 64 $\times$ 64 on the training views and enable the perceptual loss with the perceptual set to 0.1 until the end of the training procedure.

\subsection{Animation Details}
\hspace{0.422cm}We utilize depth-guided sampling benefiting from the results of geometric avatars. 
Given a novel pose, we first obtain the SMPL model and allocate a sparse volume with a resolution of 128 $\times$ 128 $\times$ 128 that contains the posed SMPL.
Then, we predict SDF values of voxels near the SMPL surface to
extract the geometric avatar using Marching Cubes~\cite{we1987marching}.
With the explicit geometric result, we can render it to the camera view to obtain a depth map.
In the following volume rendering, we can use depth-guided sampling, which means we only need to evaluate the colors of pixels inside the body mask on the depth map. 
However, the depth maps may be inaccurate on boundaries
of self-occluded regions, producing background colors. For these pixels, we re-sample points within the balls generated by SMPL vertices similar to~\cite{liu2021neural}.
Such a strategy can remarkably improve the rendering speed and it can take around 6 seconds to render the human appearance at a resolution of 1150 $\times$ 1330.

For sequential animation, e.g., the animation results shown in the supplementary video, we use a sliding window of length 5 to consider embeddings of adjacent frames in order to guarantee the temporal consistency of the results.

\begin{figure}[htb]
  \centering
  %\fbox{\rule{0pt}{2.5in} \rule{0.9\linewidth}{0pt}}
  %\includegraphics[scale=0.1]{fig/pipeline_07(1).jpg}
  \includegraphics[width=0.92\linewidth]{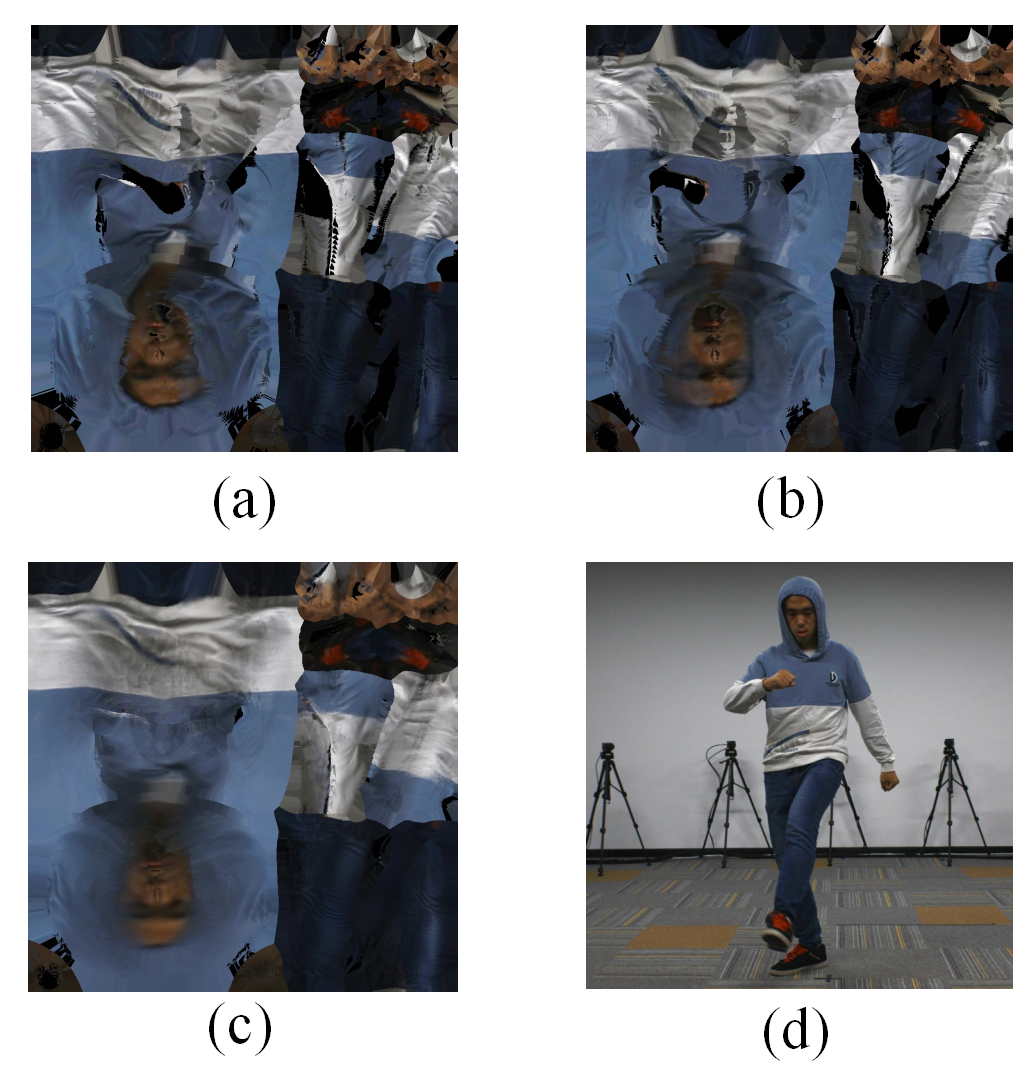}
   \caption{Image (d) and corresponding texture maps using 3 views(a), 4 views(b) and dense views(c). }
   \label{fig:fig11}
\end{figure}

\begin{figure*}[htb]
  \centering
  %\fbox{\rule{0pt}{4.5in} \rule{0.9\linewidth}{0pt}}
  %\includegraphics[scale=0.1]{fig/pipeline_07(1).jpg}
  \includegraphics[width=0.85\linewidth]{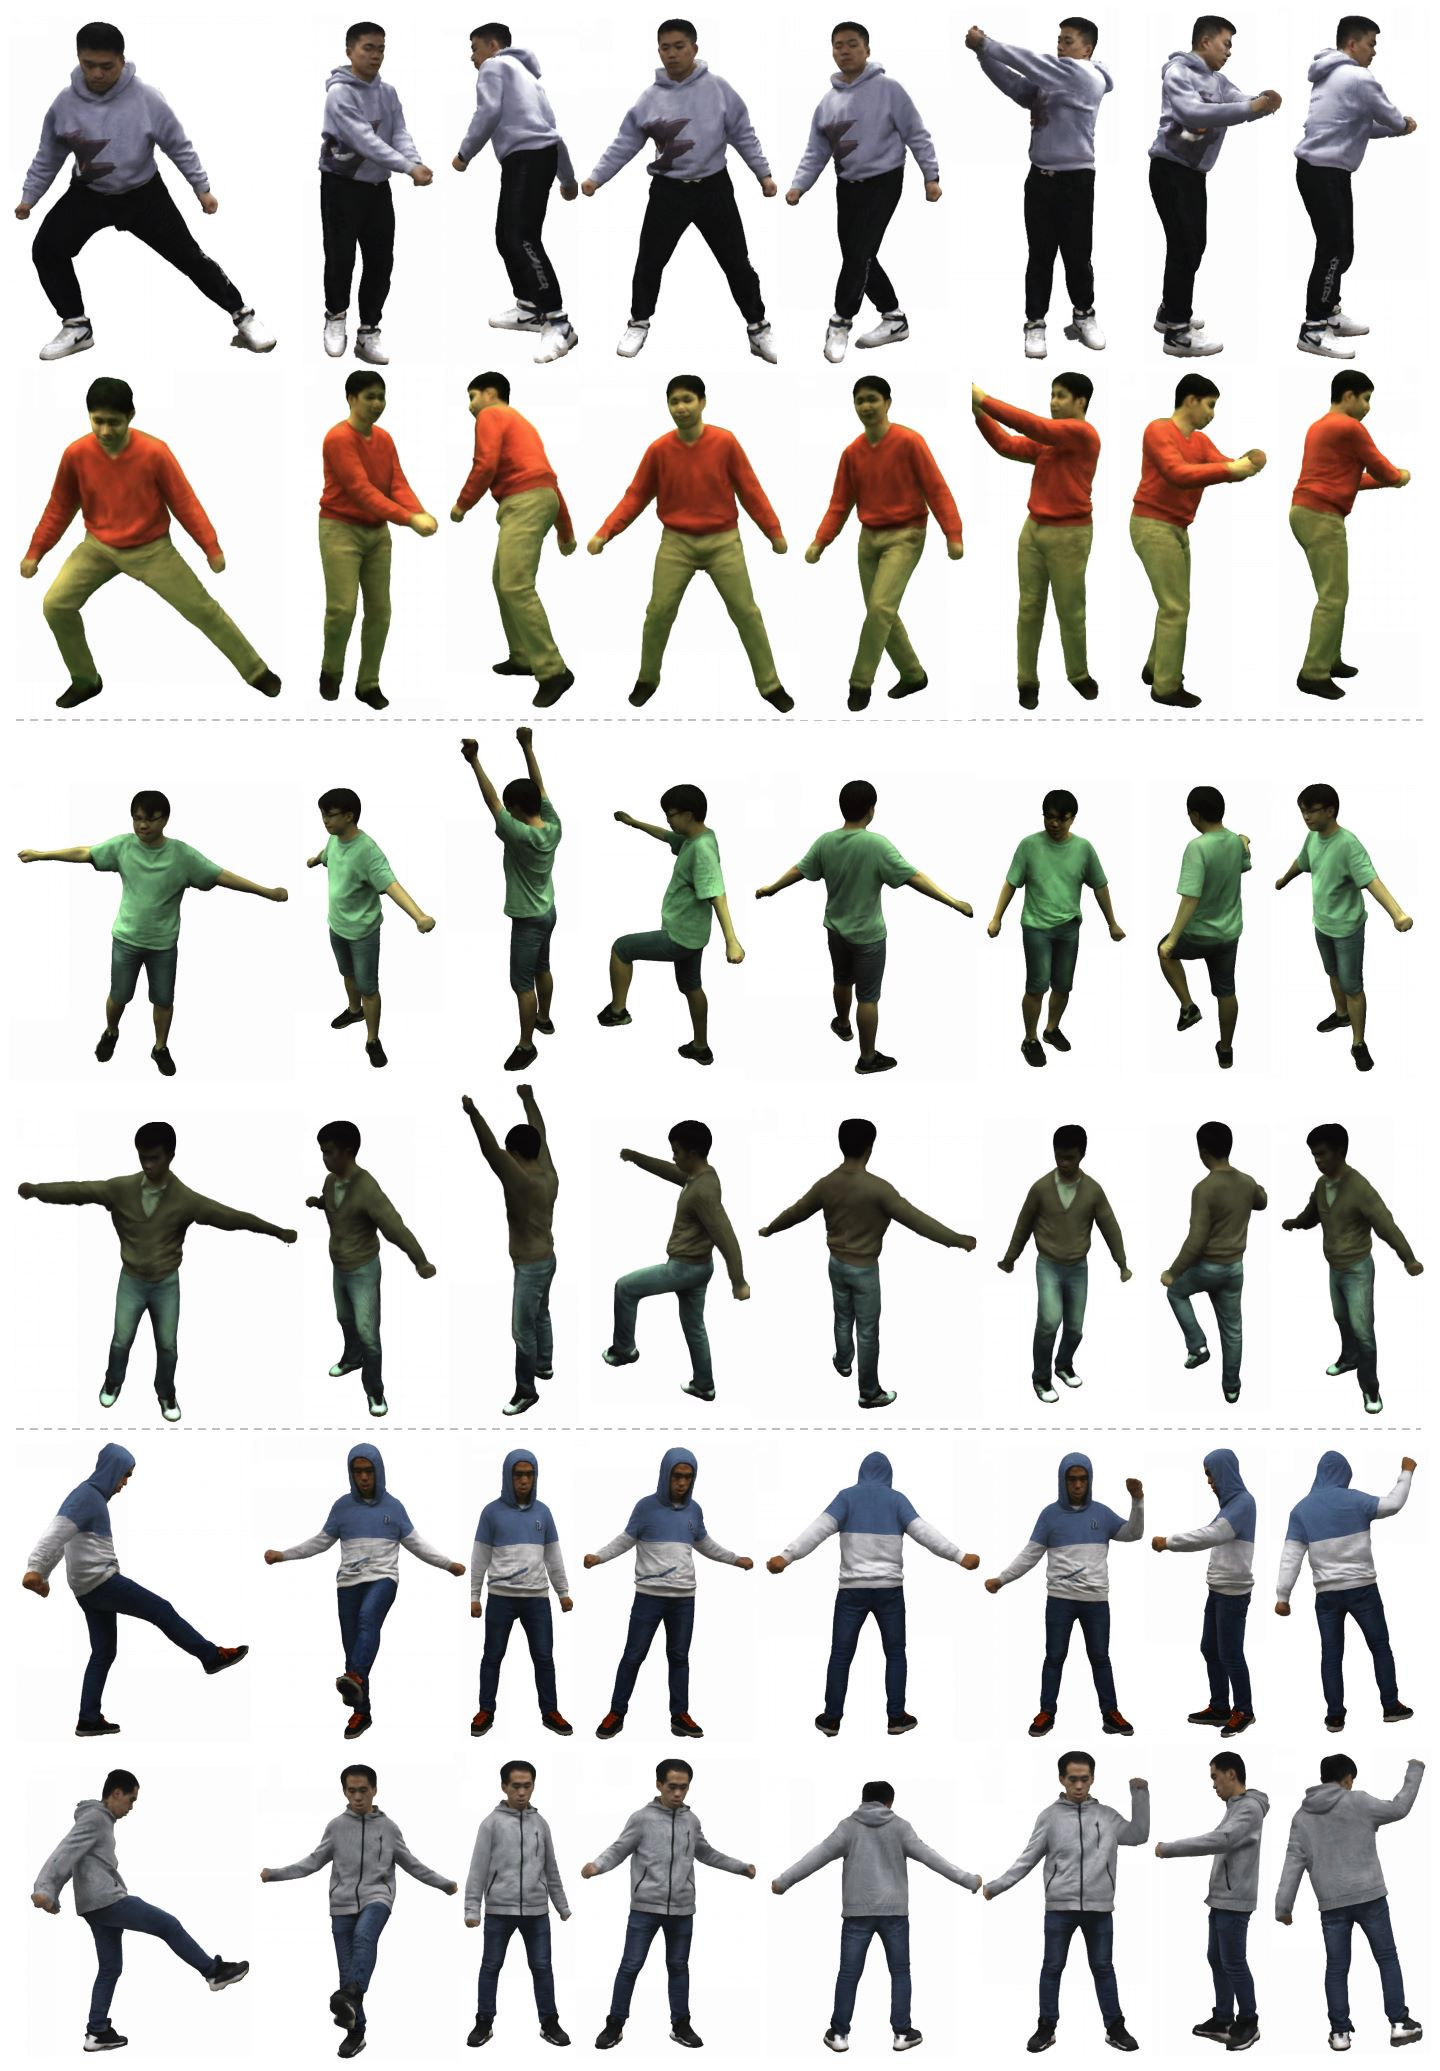}
   \caption{Animation examples on 6 sequences of multi-view videos. }
   \label{fig:figX1}
\end{figure*}

\begin{figure*}[htb]
  \centering
  %\fbox{\rule{0pt}{2.5in} \rule{0.9\linewidth}{0pt}}
  %\includegraphics[scale=0.1]{fig/pipeline_07(1).jpg}
  \includegraphics[width=0.94\linewidth]{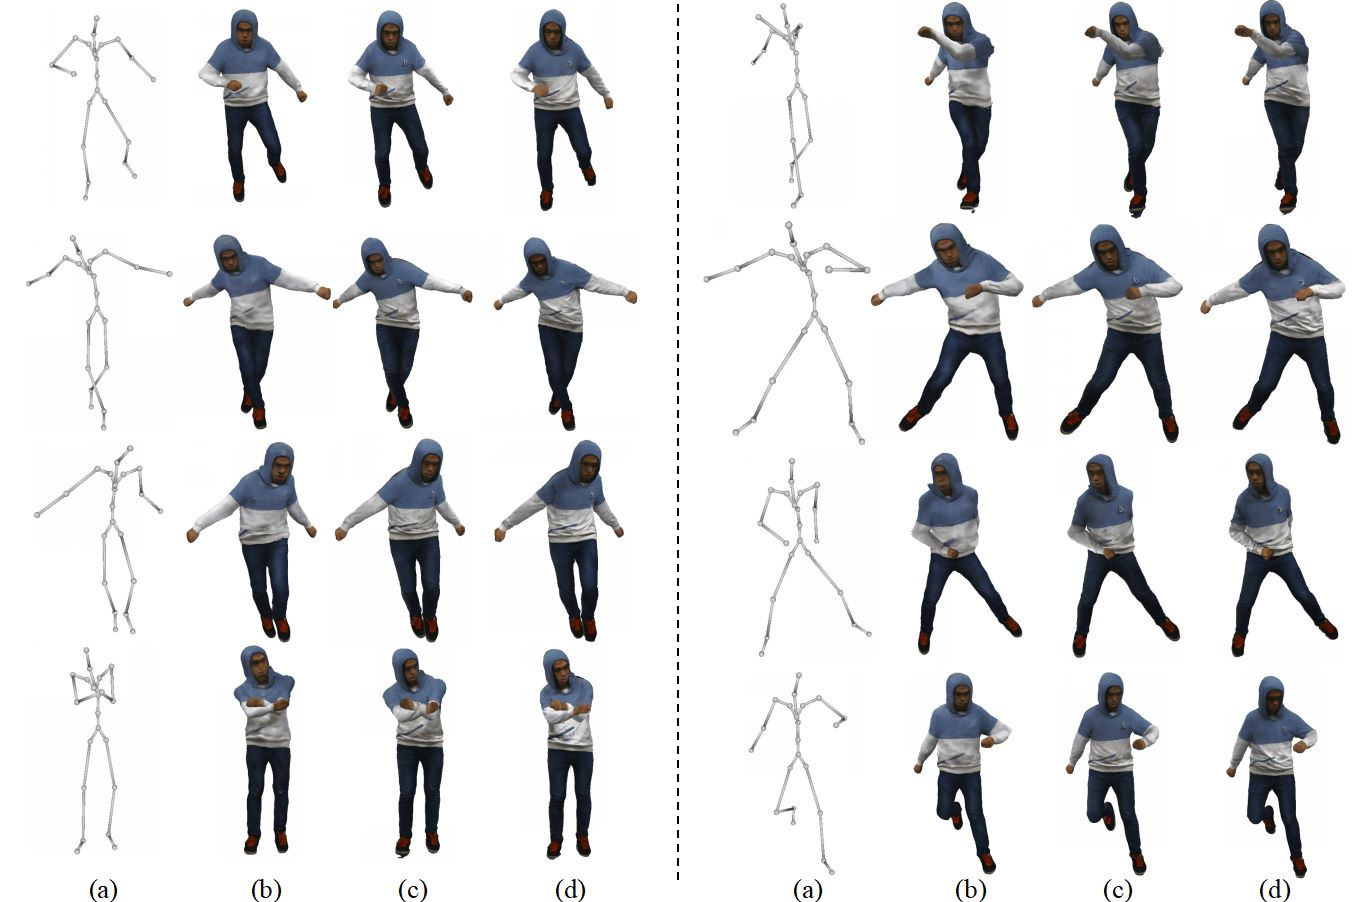}
   \caption{Animation results on AIST++~\cite{li2021ai} dataset. We compare our animation results against results produced by NeRF with Pose, and PoseVocab.(a) Driving poses, (b) NeRF MLP with pose, (c) Posevocab, (d) ours.}
   \label{fig:figX2}
\end{figure*}

\begin{figure*}[htb]
  \centering
  %\fbox{\rule{0pt}{2.5in} \rule{0.9\linewidth}{0pt}}
  %\includegraphics[scale=0.1]{fig/pipeline_07(1).jpg}
  \includegraphics[width=0.94\linewidth]{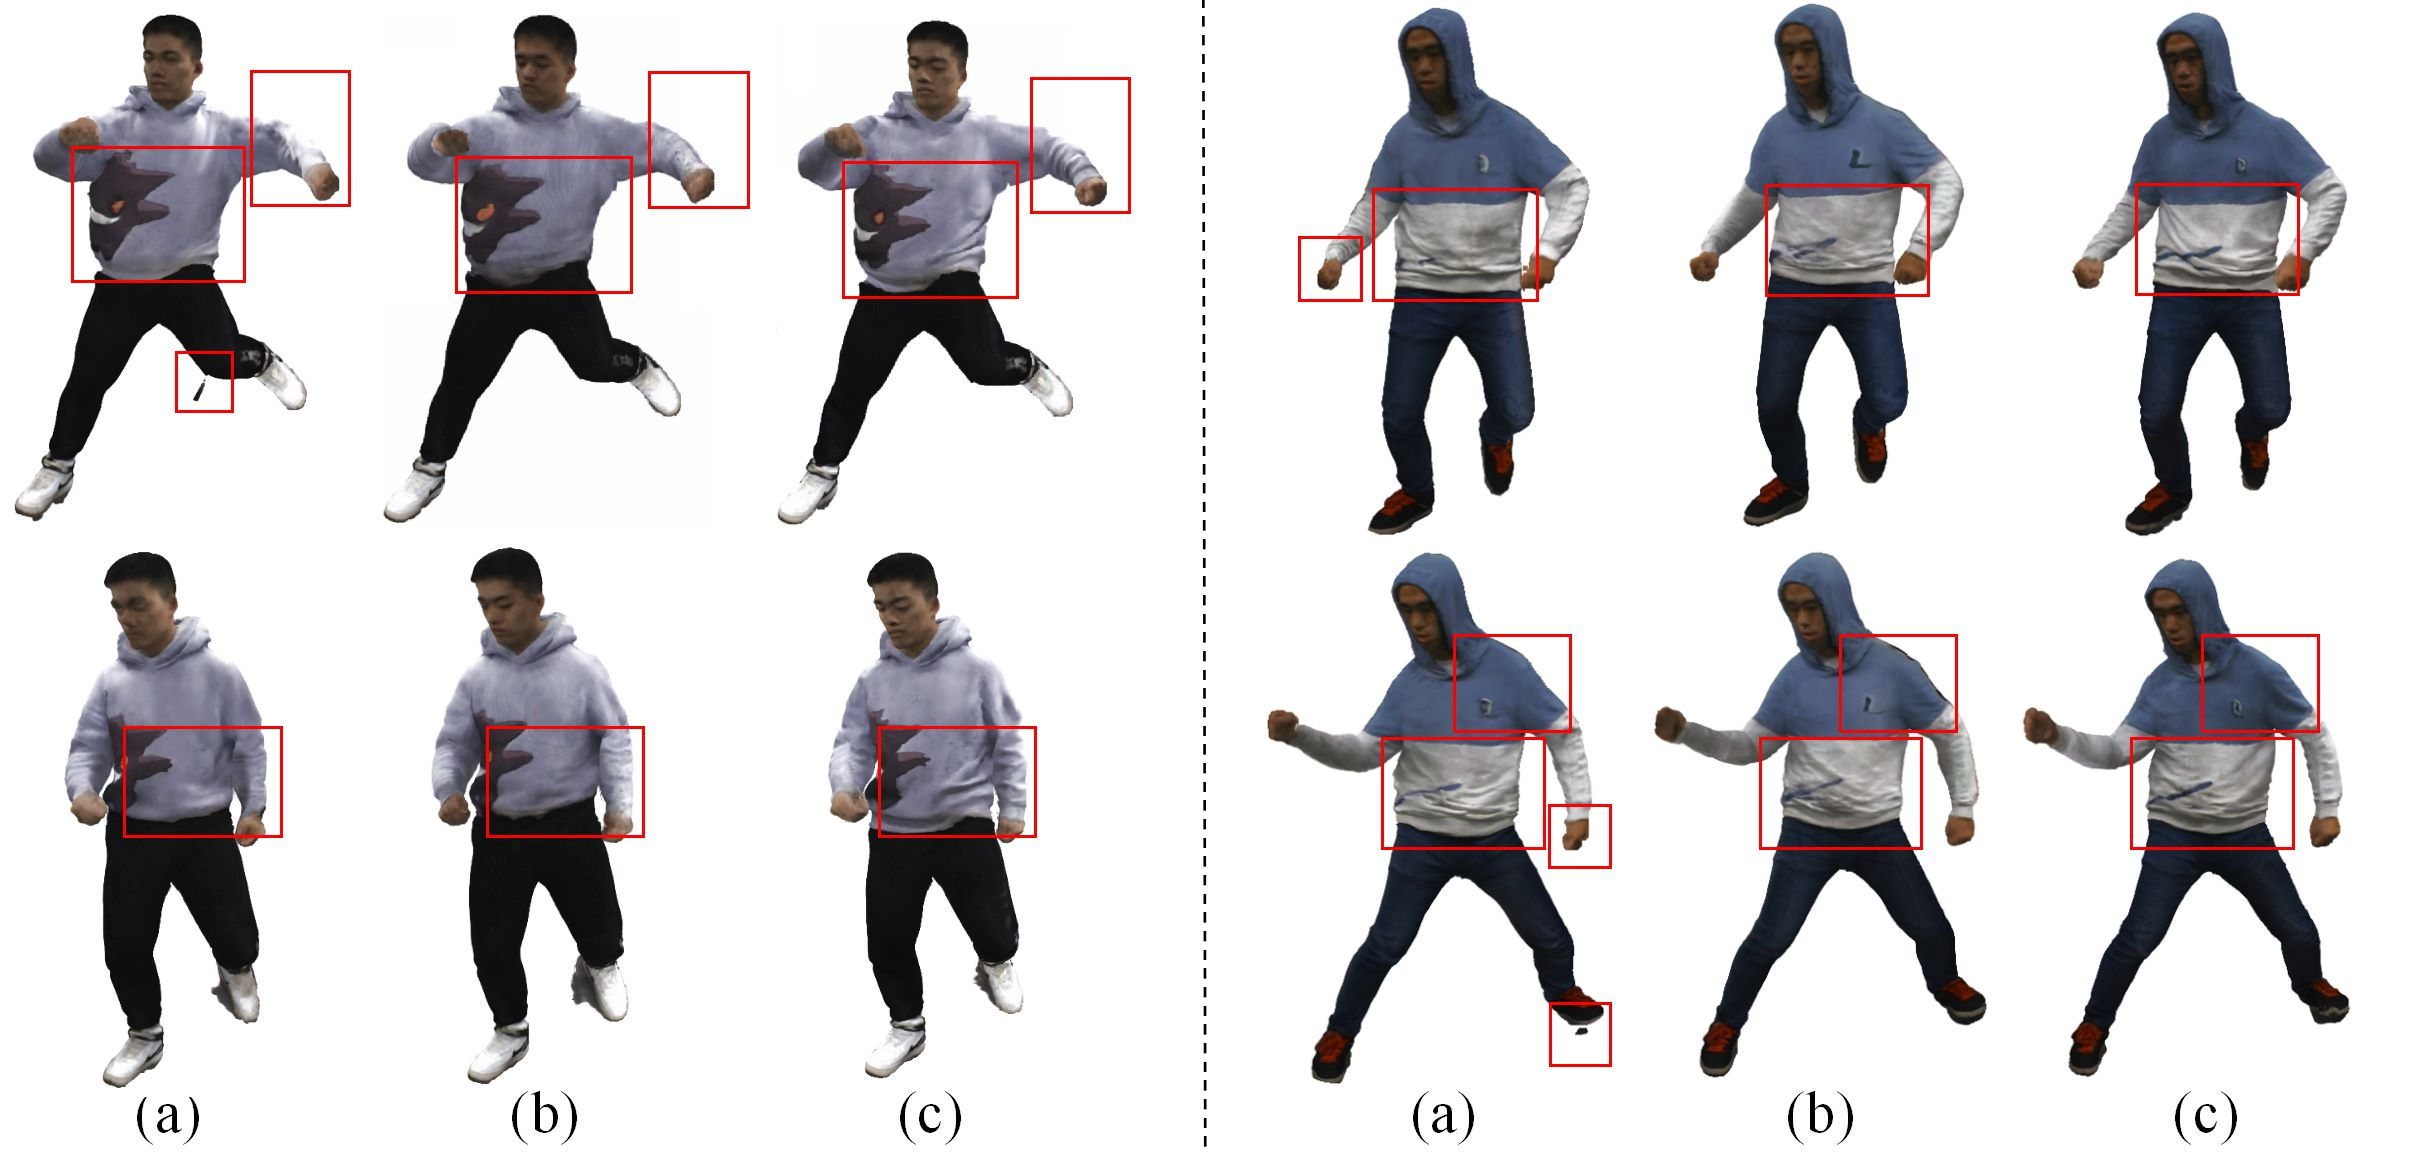}
   \caption{Animation results on AMASS~\cite{li2021ai} dataset. We compare our animation results against different encoding strategy. We show synthesized images of (a) global pose, (b) joint-structured, and (c) body-part-wise embedding.}
   \label{fig:figX3}
\end{figure*}

\section{Limitations and Future Work}
\hspace{0.422cm}In this section, we further discuss the limitations of our method and the future work.

{\bf Temporal robustness.} Actually, our method loses some temporal consistency compared with PoseVocab~\cite{li2023posevocab}. This is because the KNN neighbors in the query cannot be guaranteed to be temporally continuous. Our method and PoseVocab both suffer from this, but the values of feature lines of PoseVocab can be optimized to lie in a small range, thus producing more stable temporal animation. In contrast, the texture features in our method are of much higher frequency, yielding occasional temporal flickers sometimes.

{\bf Sparse Views.} The back-projection in Sec.4.2 relies on dense views of multi-view videos. As shown in Fig.~\ref{fig:fig11}, the texture maps might be incomplete using 3 or 4 views because of the occlusion. For instance, when the arm is placed in front of the body, part of the body may be occluded.

{\bf Body Template and Loose Clothes.} When we back-project the image evidence, we use a naked SMPL instead of a person-specific template. Since there are differences between SMPL and clothed humans, as shown in Fig.~\ref{fig:fig11}(c), the cloth pattern (specifically, the “D” letter on the hoodie) may be distorted after back-projecting. Also, the usage of SMPL UV parameterization in back-projection constrains the character to wear tight clothes, our approach cannot handle the loose clothes like long dresses. The problem may be dealt with a person-specific parametric template like~\cite{li2023animatable} instead of a sole SMPL mesh. And we leave it for future work.
